# Supplementary material for: Ultraviolet-induced fluorescence of poly(methyl methacrylate) compared to 1,1,4,4-tetraphenyl-1,3-butadiene down to 4 K
Source: arXiv:2112.11581 source file (2021-12-21)
Supplement: Supplementary file 1 [file Appendices.tex]

%\iffalse

\clearpage

\section{Remove all that follows before submission}

\subsection{List results of paper}
\begin{itemize}
    \item{Spectra and time-resolved measurements of TPB and RPT fluorescence under 285~nm excitation.}
    \item{Well-resolved spectra of TPB have been obtained down to low temperatures.  They are consistent with the literature.}
    \item{RPT spectra have been obtained as well showing TPB fluorescence.  Qualitatively, LY increases as sample cooled.}
    \item{Time-resolved LY of TPB increases as cooled in a manner concistent with literature (Francini)}
    \item{Time-resolved LY of RPT also increases as sample cooled, thought remains less than 0.5\% of TPB (at 300~K, a bit higher than Araujo which excited at shorter wavelength).}
    \item{Shape of time-resolved measurements for TPB and RPT dominated by 10~ns instrument response.}
\end{itemize}

\section{Methods}
\begin{itemize}
    \item At Troom TPB measured with 2 LED voltages, one the same as RPT (and pyrene) 13.7~V (also same as Jasmine), and a lower one for TPB (13.4~V).
\end{itemize}

\textcolor{red}{\section{Derivations}}
\todo[inline, color = jasmine]{General formatting/proofreading needed}

This model is based on~\cite{CHIRIKOVZORIN2001310}.

Let's proof some useful equation, using binom of Newton: 

\begin{equation}
\sum_{m=0}^n  \frac{a^m b^{n-m}}{m! (n-m)!} = \frac{1}{n!} \sum_{m=0}^n C_n^m a^m b^{n-m} = \frac{(a+b)^n}{n!}
\label{eq:bin}
\end{equation}

Let's proof, that convolution of two Poisson distributions with averages \(\lambda_1\) and \(\lambda_2\) is Poisson distribution with average \(\lambda_1+\lambda_2\):
\begin{equation}
(P(\lambda_1) \otimes P(\lambda_2))_n = P_n(\lambda_1+\lambda_2)
\label{eq:conv}
\end{equation}
From definition of convolution of discrete functions we find:
\[(P(\lambda_1) \otimes P(\lambda_2))_n = \sum_{m=-\infty}^\infty P_m(\lambda_1) \cdot P_{n-m}(\lambda_2)\].
Because negative indexes of Poisson distribution don't exist, previous equation will be modified:
\[(P(\lambda_1) \otimes P(\lambda_2))_n = \sum_{m=0}^n P_m(\lambda_1) \cdot P_{n-m}(\lambda_2)\].
At last, using equation (\ref{eq:bin}), we can find:
\[(P(\lambda_1) \otimes P(\lambda_2))_n = \sum_{m=0}^n \frac{e^{-\lambda_1} \lambda_1^{m}}{m!} \cdot \frac{e^{-\lambda_2} \lambda_2^{n-m}}{(n-m)!} = \sum_{m=0}^n \frac{e^{-(\lambda_1+\lambda_2)} \lambda_1^{m}\lambda_2^{n-m}}{m!(n-m)!} = \frac{e^{-(\lambda_1+\lambda_2)} (\lambda_1+\lambda_2)^n}{n!} = P_n(\lambda_1+\lambda_2)\]

Let's consider low intensity flashes directed on the PMT photo-cathode. Probability to obtain n photoelectrons from the photo-cathode can be described by Poisson distribution, where m is average number of photoelectrons per flash event:
\begin{equation}
P_{n}(m)= \sum_{n=0}^\infty  \frac{e^{-m} m^{n}}{n!}
\label{eq:pe}
\end{equation}
Then the photoelectrons hit the first dynode. Probability to obtain \(k_1\) secondary electrons produced by one incident photoelectron can be described by Poisson distribution as well, where k is average number of secondary electrons per one photoelectron:
\begin{equation}
P_{k_1}(k)= \sum_{k_1=0}^\infty  \frac{e^{-k} k^{k_1}}{k_1!}
\label{eq:se}
\end{equation}
If n photoelectrons simultaneously hit the first dynode, probability to obtain \(k_1\) secondary electrons can be found as convolution of n equations (\ref{eq:se}). Using equations (\ref{eq:se}) and (\ref{eq:conv}), we find:
\begin{equation}
P_{k_1}(k, n)= \sum_{k_1=0}^\infty  \frac{e^{-k \cdot n} (k \cdot n)^{k_1}}{k_1!}
\label{eq:mse}
\end{equation}
Also, due to semitransparency of the photocathode, some photons hit the first dynode instead the photocathode and produce first dynode photoelectrons. Probability to obtain \(n_1\) first dynode photoelectrons can be described by Poisson distribution, where \(m_1\) is average number of first dynode photoelectrons per event:  
\begin{equation}
P_{n_1}(m_1)= \sum_{n_1=0}^\infty  \frac{e^{-m_1} m_1^{n_1}}{n_1!}
\label{eq:fdpe}
\end{equation}
As we know from equations (\ref{eq:mse}) and (\ref{eq:fdpe}), \(k_1+n_2\) electrons hit the second dynode in certain event. Usually this number is big enough to consider response of the dynode system with exception of the first dynode like Gaussian:
\begin{equation}
G(x, c, \sigma)=\frac{1}{\sqrt{2 \pi \sigma^2}} exp(\frac{(x-c)^2}{2 \sigma^2})
\label{eq:Gauss}
\end{equation}
where x is charge collected on the PMT anode as a response on flash event, and \( c= x_0+(k_1+n_1)x_1\), and \(\sigma^2 =  s_0^2+(k_1+n_1)s_1^2\), \(x_0\) - pedestal, average charge collected in absence of light; \(x_1\) - average charge, collected by the dynode system without the first dynode per one electron; \(s_0\)-standard deviation of the pedestal; \(s_1\) - standard deviation of single electron response of the dynode system without the first dynode.
At last, using equations (\ref{eq:pe}), (\ref{eq:mse}), (\ref{eq:fdpe}), and (\ref{eq:Gauss}), we find the final equation (\ref{eq:Sr}), describing integral distribution of spe spectra.

\newpage

\section{Pulser Circuit Tests}
The UV irradiation stability tests were done. For this the RPT sample at room temperature 291 K was irradiated with UV light and the light yield was detected similarly to the main experiment. The light yield was measured every day during a week.The RPT sample luminescence efficiency is supposed to be the same at the same temperature, so difference in the detected light yield is attributed to instability of the pulser circuit. The results of the measurement are shown in table \ref{tab:Tab_room temp_tests}. In the first column the day of measurement is shown. In the second column the detected light yield in average number of photoelectrons and error of fit are shown. It is seen in the table \ref{tab:Tab_room temp_tests}, that first three measurements made immediately one after one show the same result within error of fit. The measurements made while the week show average light yield 0.385 photoelectrons with standard deviation 5 \%.

\begin{table}[H]
    \centering

\begin{tabular}{ll}
 \hline
Day & Detected light yield \\
1   & 0.418$\pm$0.002   \\
1   & 0.420$\pm$0.002   \\
1   & 0.418$\pm$0.002   \\
2   & 0.396$\pm$0.002   \\
3   & 0.373$\pm$0.002   \\
4   & 0.379$\pm$0.002   \\
6 morning   & 0.365$\pm$0.002   \\
6 night & 0.373$\pm$0.002   \\
7   & 0.386$\pm$0.002   \\
\end{tabular}
    \caption{\label{tab:Tab_room temp_tests}Detected light yields at room temperature obtained at different time}
\end{table}

\clearpage

\section{SPE response tests (Hicham)}

\subsection{Average SPE charge}

In the conditions of the experiment, luminescence from RPT sample has relatively low amplitude and is mainly composed of just a few photoelectrons. Then, the number of photoelectrons can be easily calculated thanks to the fit of RPT integral distribution with the function described in Sec.~\ref{sec3}. Fitted 300K RPT integral distribution can be observed on Fig.~\ref{fig:RPT_dist_0p1}.

\begin{figure}[H]
    \centering
    \includegraphics[width=1.0\textwidth]{RPT/RPT2_LED285nm_300K_9401_Ch0_distr(870-920 ns).pdf}
    \caption{RPT integral distribution - \(\pm\)0.1V vertical scale}
    \label{fig:RPT_dist_0p1}
\end{figure}

On Fig.~\ref{fig:RPT_dist_0p1}, a parameter called m can be calculated. It represents the average number of photoelectrons detected per event on the chosen integration window. Here, it means that in average, 0.397 photoelectrons per event are detected by the PMT on the chosen integration window.

Since TPB sample emits a lot of photoelectrons at the same time, it is more complicated to determine precisely the amount of light emitted. For TPB indeed, it is necessary to know the charge of one single photoelectron (SPE), charge that depends on the PMT used. It will let us know the number of photoelectrons emitted by a sample at one temperature and let us analyze the variations of it with temperature. To do that experimentally, we decreased the voltage of the LED until the TPB response was low enough to get single photoelectrons detected by the PMT. These low emission response runs from TPB were called TPB SPE.

Since TPB SPE runs have a weak luminescence (like RPT runs), we were able to fit the integral distribution of these runs with the function described in Sec.~\ref{sec3}. The average of the integral distribution will give the integral value of an SPE for this run. On Fig.~\ref{fig:TPB2SPE_dist}, we have an example of a fitted distribution for a TPB SPE run at room temperature on \(\pm\) 2V.

\begin{figure}[H]
    \centering
    \includegraphics[width=0.8\textwidth]{TPB/TPB2SPE_LED285nm_300K_9301_Ch0_distr(470-530 ns).pdf}
    \caption{TPB SPE integral distribution - \(\pm\)2V vertical scale}
    \label{fig:TPB2SPE_dist}
\end{figure}

For this distribution, the SPE integral value was found to be equal to $1.42 \pm 0.07$~ADU$\mu$s. This will be the value used in our analysis to determine the number of photoelectrons emitted by the TPB sample.

\subsection{Stability on different scales}

Since TPB runs have mainly been done on \(\pm\) 2V vertical scale, only SPE integral value on \(\pm\) 2V scale is necessary to get the number of photoelectrons emitted. However, it can be interesting to study the stability of this SPE value on different vertical scales. This is why TPB SPE data have been recorded on five different scales.

Fig.~\ref{fig:TPB_SPE_dist_0p1} and Fig.~\ref{fig:TPB_SPE_dist_2p5} show two fitted TPB SPE integral distributions respectively on \(\pm\) 0.1V and \(\pm\) 2.5V.

\begin{figure}[H]
    \centering
    \includegraphics[width=0.8\textwidth]{Analysis/TPB2_LED280nm_11V_0p1_Ch0_distr(110-160 ns).pdf}
    \caption{TPB SPE integral distribution - \(\pm\)0.1V vertical scale}
    \label{fig:TPB_SPE_dist_0p1}
\end{figure}

For this distribution, the SPE integral value was found to be equal to 32.795 ADU$\mu$s.

\begin{figure}[H]
    \centering
    \includegraphics[width=0.8\textwidth]{Analysis/TPB2_LED280nm_11V_2p5_Ch0_distr(110-160 ns).pdf}
    \caption{SPE integral distribution - \(\pm\)2.5V }
    \label{fig:TPB_SPE_dist_2p5}
\end{figure}

On this scale, the integral distribution shape is different and we get a SPE integral value of 1.335 ADU$\mu$s. On Tab.~\ref{tab:Tab_SPE_scale}, all SPE integral values are compiled for these different vertical scales.

\begin{table}[H]
    \centering

\begin{tabular}{ll}
 \hline
Vertical scale (V) & Average SPE integral (ADU$\mu$s) \\
$\pm$ 0.1                & 32.795$\pm$0.567               \\
$\pm$ 0.2                & 13.236$\pm$0.201               \\
$\pm$ 0.5                & 6.47$\pm$0.149                 \\
$\pm$ 1.0                & 3.347$\pm$0.077                \\
$\pm$2.5                & 1.335$\pm$0.067               
\end{tabular}
    \caption{\label{tab:Tab_SPE_scale}Average SPE integral on different vertical scales}
\end{table}

Since conversion constants for each scale are known, after conversion of the SPE integral from ADU$\mu$s to V*s, we can compare these values for the five different scales. Fig.~\ref{fig:Scale_test_spe} shows this spe average charge for these five scales.

\begin{figure}[H]
    \centering
    \includegraphics[width=0.7\textwidth]{Analysis/Scale_test_spe.pdf}
    \caption{Scale test for average SPE charge}
    \label{fig:Scale_test_spe}
\end{figure}

Fig.~\ref{fig:Scale_test_spe} shows pretty similar values of SPE charge for each vertical scale, then average SPE charge is consistent whatever the scale is.

Also, from Fig.~\ref{fig:TPB_SPE_dist_0p1} and Fig.~\ref{fig:TPB_SPE_dist_2p5}, the average number of photoelectrons detected per event on the chosen integration window, m, has been calculated. $m = 0.115$ for example means that every event shows in average 0.115 photoelectrons on the integration window. Fig.~\ref{fig:Scale_test_LY} shows the values of this number of photoelectrons for different vertical scales.

\begin{figure}[H]
    \centering
    \includegraphics[width=0.7\textwidth]{Analysis/Scale_test_LY.pdf}
    \caption{Scale test for average number of photoelectrons per event}
    \label{fig:Scale_test_LY}
\end{figure}

Fig.~\ref{fig:Scale_test_LY} shows pretty similar values for each vertical scale, which proves the stability of the runs for different vertical scales.

\subsection{Average SPE trace}

It can also be looked at the average amplitude of an event in different runs. First, we can compare RPT run (low number of photoelectrons - SPE run) and TPB SPE run average pulse shapes. These two runs were measured on pulse \(\pm\)2V scale and have been normalized to have a main pulse amplitude equal to 1. A cut has been made for noise with low integral values. These two pulse shapes are plotted on Fig.~\ref{fig:pulseshape1}. Pulse shapes have been smoothed with an elliptic filter to get rid of LED induced noise.

\begin{figure}[H]
    \centering
    \includegraphics[width=0.7\textwidth]{Analysis/pulseshapes1.png}
    \caption{Average pulse shape for TPB SPE run (blue) vs RPT run (orange) - \(\pm\)2V scale}
    \label{fig:pulseshape1}
\end{figure}

If we compare these two runs, we can see that main part of both peak overlay each other or are very close, so it can be interpreted as two very similar pulse shapes. Differences between both plots can be understood as random variations of LED induced noise if we take into account the fact that noise is relatively important on these runs and we can't get rid of it completely with the filter.

Also, we can compare the pulse shape from the RPT runs and a LED SPE run - which is a SPE run without sample, the LED pulsing directly on the PMT. The two plots are showed on Fig.~\ref{fig:pulseshape2} after a cut made on low-integral pulses (noise pulses).

\begin{figure}[H]
    \centering
    \includegraphics[width=0.7\textwidth]{Analysis/pulseshapes2.png}
    \caption{Average pulse shape for LED SPE run (blue,  $\pm 0.2$~V scale) vs RPT run (orange, $\pm 2$~V scale)}
    \label{fig:pulseshape2}
\end{figure}

On Fig.~\ref{fig:pulseshape2}, we can see that rise time of main peaks are very similar - a little faster without sample. 

Then, we can compare these previous runs with TPB run average shape with a higher voltage. This TPB run is not a SPE run as many photoelectrons are detected by the PMT simultaneously. The average shape maximum amplitude from this run was normalized to be equal to 1. After a noise cut, these average pulse shapes are showed on Fig.~\ref{fig:pulseshape3}.

\begin{figure}[H]
    \centering
    \includegraphics[width=0.7\textwidth]{Analysis/pulseshapes3.png}
    \caption{Average pulse shape for TPB SPE run (blue) vs LED SPE run (orange) vs RPT run (green) vs TPB run (red) - \(\pm\)2V scale}
    \label{fig:pulseshape3}
\end{figure}

We can see on Fig.~\ref{fig:pulseshape3} that TPB run average pulse shape has the same rise time and same width as other runs made before. We understand with this study that, no matter the sample, the LED voltage or the number of photoelectrons detected by the PMT, all average pulse shapes are very similar.

\section{influence of integration window (TPB)}

\begin{figure}[H]
    \centering
    \includegraphics[width=0.7\textwidth]{integral/TPB3_LED285nm_87K_107_01int_mean_plus.pdf}
    \caption{Average pulse shape of TPB at 87 K in log scale (top). Integral mean value (from skew normal distribution fit) for different upper limit of the integration window (bottom).}
    \label{fig:int_window_TPB}
\end{figure}

\begin{figure}[H]
    \centering
    \includegraphics[width=0.7\textwidth]{integral/TPB3_LED285nm_87K_107_01int_distri.pdf}
    \caption{Integral distribution of TPB at 87 K and skew normal distribution fit for different upper limit of integration window.}
    \label{fig:int_distri_TPB}
\end{figure}

\section{Justifying the correction factor (Philippe)}

At each temperature $T$, we measure $\frac{n_{RPT}(T; 13.7)}{ n_{TPB}(T; 13.4)}$, and we want $\frac{n_{RPT}(T; 13.7)}{ n_{TPB}(T; 13.7)}$.  These are related by:

$\frac{n_{RPT}(T; 13.7)}{ n_{TPB}(T; 13.7)} = \frac{n_{RPT}(T; 13.7)}{ n_{TPB}(T; 13.4)} \frac{n_{TPB}(T; 13.4)}{n_{TPB}(T; 13.7)}$

We measure the term $ \frac{n_{TPB}(T; 13.4)}{n_{TPB}(T; 13.7)}$ at room $T$, and assume it does not depend on temperature.  This is plausible since $n_{TPB}(T; 13.4)$ only varies by $\sim  25\%$ over the range of temperatures.

\section{Errors (Quentin)}\label{app:errors}

Errors on skew normal distribution mean :\\
\begin{equation}
    \Bar{m}(k,z,a)=k+\sqrt{\frac{2}{\pi}}z \frac{a}{\sqrt{1+a^2}}~~;~~k~location,~z~scale,~a~shape.
\end{equation}

\begin{equation}
    {\Delta \Bar{m}}=\sqrt{(\Delta k)^2 + \left(\sqrt{\frac{2}{\pi}} \frac{a}{\sqrt{1+a^2}} \Delta z \right) ^2 + \left(\sqrt{\frac{2}{\pi}} z \frac{1}{(1+a^2)^{\frac{3}{2}}} \Delta a \right)^2}
\end{equation}

Errors details for Table \ref{tab:tpb_cor_factor} at 300~K :

\begin{table}[h]
    \centering
    \begin{tabular}{|c|c|c|}
    \hline
    LED voltage & Integral mean (adu.µs) & Integral mean (SPE)\\
    \hline
    13.4 V & 92.44 \pm~ 0.3118 & 66.985 \pm~ 0.2979 \\
    \hline
    13.7 V & 236.235 \pm~ 0.1943  & 171.18 \pm~ 0.5158 \\
    \hline
    \hline
    correction factor & 2.555 \pm~ 0.009 \\
    \hline
    \end{tabular}
    \caption{The values and errors of the integral mean in adu.µs come from the fit. The ones in SPE are obtained using an SPE integral value of 1.380 $\pm$ 0.004  adu.µs (the errors are calculated using error propagation of a ratio). The correction factor is obtained by dividing the value at 13.7 V and those at 13.4 V.}
    \label{tab:error_details}
\end{table}

Details conversion from adu.µs to SPE :\\
\begin{multline*}
    92.44  ~\pm  ~0.3118 ~\text{adu.µs} = \frac{92.44}{1.38} ~ \pm ~ \sqrt{\left(\frac{0.3118}{1.38}\right)^2+\left (\frac{92.44 \times 0.004}{1.38^2}\right)^2}~\text{SPE}=66.985 ~ \pm ~ 0.2979~ \text{SPE}\\
    \\
    236.235  ~\pm ~ 0.1943 ~\text{adu.µs} = \frac{236.235}{1.38} ~ \pm ~ \sqrt{\left(\frac{0.1943}{1.38}\right)^2+\left (\frac{236.235 \times 0.004}{1.38^2}\right)^2}~\text{SPE}=171.18 ~ \pm ~ 0.5158~ \text{SPE}
\end{multline*}

\subsection{Error on ratio (Philippe)}
If $z=x/y$, then $\ln z = \ln x - \ln y$ and $\delta z/z = \delta x /x - \delta y /y$.  Assuming fluctuations are independent and adding quadratically: $\sigma_z^2 / z^2 = \sigma_x^2 / x^2 + \sigma_y^2 / y^2$ so $\sigma_z^2 = \sigma_x^2 / y^2 + x^2 \sigma_y^2 / y^4$

\subsection{RPT Light Yield Errors}
The systematic errors for RPT were determined by calculating the light yields using different length integration windows for the light yield, keeping the start of the window at the same point and changing the upper bound. Fig.~\ref{fig:rpt_bounds} is the result of these calculations where the same data set of RPT at 87~K was reanalyzed with different integration windows. 
\begin{figure}[H]
\begin{center}
\includegraphics[width=0.6\textwidth]{light_yield/rpt_changing_bounds.pdf}
\caption{\label{fig:rpt_bounds}Change in the RPT light yield with different upper limits on the integration window (at 87~K).}
\end{center}
\end{figure}

The light yield with a 50~ns window was 0.860~pe while it was 0.899~pe with a 480~ns window. The 480~ns integration window light yield was the largest deviation from the light yield observed for the usual 50~ns window. Taking the difference of these values as an estimate of the systematic uncertainty on the light yield of RPT at 87~K it works out to 0.039~pe. This value will likely scale with the light yield so we express the systematic uncertainty as a percentage of the light yield. With an estimate of the systematic uncertainty at 87~K as 0.039~pe and LY(87~K) = 0.860~pe, we set the systematic uncertainty for RPT in general as $\Delta LY_{RPT,sys} = 5\%$.

The statistical uncertainty for the RPT light yield measurements comes directly from the mean of the fit models introduced in subsection~\ref{sec:LY} as fitting with those single photoelectron distribution makes everything already in terms of the number of photoelectrons. The overall uncertainty in the RPT light yield is a combination of the statistical and systematic uncertainties according to Eq.~\ref{eq:rpt_ly_uncertainty}

\begin{center}
\begin{equation}
    \Delta LY_{RPT} = \sqrt{\Delta LY_{RPT,sys}^2 + \Delta LY_{RPT,stat}^2} 
    \label{eq:rpt_ly_uncertainty}
\end{equation}
\end{center}

\subsection{TPB Light Yield Errors}

For TPB there are a few additional factors to consider in addition to the analysis explained for RPT. These include a contribution to the statistical uncertainty from the correction factor for the LED voltage and a different value for the average integral for a single photoelectron due to the different digitizer vertical range for TPB. The first step is determining the uncertainty for the number of photoelectrons, before applying the correction factor. For the light yield this is $LY_{TPB,lowV} = m/1.38$ where m is the mean of the skew normal distribution and $1.38 \pm 0.0004 ADU \mu s$ is the average integral for a single photoelectron for a digitizer vertical range of $\pm$2.5~V. The uncertainty calculations for this value were summarized in a previous subsection describing the conversion from the integral in $ADU \mu s$ to number of photoelectrons according to Eq.~\ref{eq:int_to_pe}.

\begin{equation}
    \Delta LY_{TPB,lowV} = \sqrt{   \left(\dfrac{\Delta m}{1.38}\right)^2  + \left(\dfrac{m\times0.004}{1.38^2}\right)^2  } 
    \label{eq:int_to_pe}
\end{equation}

The next step is then applying the correction factor to data where it is taken as 2.5461 $\pm$ 0.0005. The total light yield $LY_{TPB,tot} = LY_{TPB,lowV} \times 2.5461$, so the overall statistical uncertainty is just from adding the relative uncertainties in quadrature.

\begin{equation}
    \left(\dfrac{\Delta LY_{TPB,stat}}{LY_{TPB,stat}}\right)^2 =  \left(\dfrac{\Delta LY_{TPB,lowV}}{LY_{TPB,lowV}}\right)^2 + \left(\dfrac{0.005}{2.5461}\right)^2
\end{equation}

The systematic errors are calculated using the same method as for RPT except that the data used was at 300~K instead of the 87~K used for RPT as shown in Fig.~\ref{fig:tpb_bounds}. 
The light yield with a 50~ns window and before applying the correction factor was 66.97~pe while it was 67.53~pe with a 2000~ns window, the window when the deviation from the light yield with the 50~ns is the greatest. The difference between these two values is the estimate of the systematic error at 300~K which is $\Delta LY_{sys}$(300~K) = 0.56~pe. Based on the ratio of the estimate of the systematic uncertainty fro the window (0.56~pe) and the light yield with the 50~ns window (66.97~pe), the systematic uncertainty $\Delta LY_{TPB,sys}$ was set to 1\% of the overall light yield according.

\begin{figure}[H]
\begin{center}
\includegraphics[width=0.6\textwidth]{light_yield/tpb_changing_bounds.pdf}
\caption{\label{fig:tpb_bounds}Change in the TPB light yield with different upper limits on the integration window (300~K).}

\end{center}
\end{figure}

Overall this takes the total light yield just adding the absolute statistical and systematic uncertainties in quadrature. 
\begin{equation}
    \Delta LY_{TPB,tot}^2 = \Delta LY_{TPB,stat}^2 + \Delta LY_{TPB,sys}^2
\end{equation}

\subsection{Relative Light Yield Errors}
The relative light yield of RPT to TPB is 
\begin{equation}
    relLY = \dfrac{LY_{RPT,tot}}{LY_{TPB,tot}}
\end{equation}
and so the uncertainty will just be adding the relative uncertainties in quadrature according to 
\begin{equation}
    \left(\dfrac{\Delta relLY}{relLY}\right)^2 =  \left(\dfrac{\Delta LY_{RPT,tot}}{LY_{RPT,tot}}\right)^2 +  \left(\dfrac{LY_{TPB,tot}}{LY_{TPB,tot}}\right)^2
\end{equation}

\section{Not for publication --- private appendices}

\subsection{Literature review (Pauline)}
TPB

 In work [15] authors measure re-emission spectra of TPB film, illuminated with 128, 160, 175, 250 nm UV light. Also they measure fluorescence efficiency of the sample as a function of incident UV light in range from 120 - 250 nm. The sample was Solacryl SUVT acrylyc from Spartech Polycast, coated with 1.5 \( \pm \) 0.05 \(\mu\)m by vacuum technology. The re-emission spectra turned out to be very similar to each other with exception of little bump after 500 nm at 128 nm UV illumination. The fluorescence efficiency was found between 0.7 and 1.35 photon emitted for each UV photon absorbed.
 
 In work [19] authors present re-emission spectra of TPB films under illumination with 45, 128, 160, 175, 250 nm UV light. Also WLSE of TPB films with different thickness from 0.7 to 3.7 \(\mu\)m are shown with TPB quantum efficiency vs incident UV light wavelength. Also absorption length of UV light in TPB is found in this work as well. The samples are made of 0.318 cm thick SUVT stock acrylic with PTB coating. The re-emission spectra were found similar to each other for different wavelengths of incident UV light. The obtained TPB quantum efficiency varies between 0.3 - 0.8 depending on wavelength of incident UV light with trend to decrease with decrease of UV light. The UV absorption length in TPB was found about 400 nm \(\pm\)150nm.
 
 In work [] authors report report about existance of long component of TPB luminescense under excitation with 128 nm UV light. They found, that time properties of the long component are the same under irradiation with different particles, but it's intensity is different. The authors report, that this long component can complicate pulse shape discrimination in LAr by distorting obtained signal.
 
 In work [20] authors report about existence of long component in TPB scintillation with length about 1 ms. They found that intensity of this long component depends on kind of excitation particle. It was found that using pulse shape discrimination, surface background suppression on DarkSide-50 experiment can be greater than \(10^3\) on window 1 ms.

In work [21] authors investigate photoluminescence and excitation spectra of samples consisting of TPB films with different thicknesses deposited on glass and polimeric substrates, and polystyrene-TPB film deposited on glass substrate. Also temperature dependence of the samples luminescence was investigated. Luminescence structure corresponding to vibrational sublevels of TPB was found at low temperature for samples with pure TPB coating. Also it was found, that TPB integral luminescence intensity increases on 10\% at the temperature going from 300 K to 87 K. 

RPT

In work [23] optical properties and autoluminescence of different materials are investigated. autoluminescence of BoroFloat glass, PMMA, PC, COC, PDMS samples was measured under 403, 488, 532, 633 nm light excitation. Plastics show much higher level of authofluorescence than BoroFloat glass. Also the highest level of autofluorescence was observed at excitation with 403 nm light. Also bleaching of authofluorescence observed.

In work [27] luminescence of PMMA under excitation with electron beam and 222 nm UV light. Samples with thicness 6 and 10 mm show broad band at 490 nm. 3mm thick sample showed additional band at 400 nm. Also Absorption spectre on 3 mm sample was shifted from 300 nm to 350 nm what can be expleined by presence of additional impurity.

In work [34] luminescence of RPT acrylic, Spartech acrylic and PTFE was investigated in range from 400 to 550 nm and at excitation in range from 130 to 250 nm at room temperature. The upper limit of Luminescence intensity was found. For PTFE it is 0.35 \% and for RPT and Spartech acrylic it is 0.2 \% relatively to TPB.

\subsubsection{More from Philippe}
\begin{description}
\item[Wallace-Williams 1994, The Journal of Physical Chemistry]{Room temperature

Fig 3: absorption spectrum of TPB

Fig 7: decay profile when excited at 295 nm and observed at 650 nm}

\item[Biller 2020, NIM]{At room temperature

Includes pyrene

Absorption is in Figure 6

Molar extinction coef is about 2E3 at 285 nm

Discusses light yield, time profile, and absorption of pyrene

Light yield about 0.65

Eq 1: Uses a 2 exp fall and 1 exp rise for excimer and for monomer}

\item[Graybill 2020, Applied Optics]{Fig 13 gives absorption coef of TPB as a function of  wavelength, up to 200 nm

6E5 /cm at 200 nm}

\end{description}

\subsection{Lit review reboot, Jonathan}
\subsubsection{TPB}

The usage of Tetraphenyl-Butadiene (TPB) as a wavelength converter from the ultra-violet to visible spectrum has been suggested since as early as 1973 from Burton \& Powell \cite{Burton}.

Various sources report an emission spectra in the visible light region upon UV irradiation which peaks at approximately 440\textit{}{nm} as reported from Burton \& Powel \cite{Burton}, Lally \cite{Lally}, Francini \cite{Francini},and Corning \cite{jasmine_lidine} as illustrated by figures~\ref{Burton Spectra}-\ref{Corning Spectra}.  The incident light's wavelengths for these four plots varied from \SI{185}{nm} to \SI{380}{nm} and the peak in emission is agreed upon by all four papers.  The study from Corning et. al. \cite{jasmine_lidine} suggests that the emission spectra is temperature dependent and changes slightly with a decrease in temperature as exhibited by fig \ref{Corning Spectra}. 

\begin{figure}[H]
\centering
\begin{minipage}{.49\textwidth}
  \centering
  \includegraphics[width=.8\textwidth]{Lit Review/Burton and Powell Fig 2.png}
  \caption{Emission spectra of TPB from \SI{253.7}{nm} light irradiation as reported by Burton \& Powel \cite{Burton}}
  \label{Burton Spectra}
\end{minipage}\hfill
\begin{minipage}{.49\textwidth}
  \centering
  \includegraphics[width=.9\textwidth]{Lit Review/Lally_fig4b.png}
  \caption{Emission spectra of TPB from \SI{185}{nm} light irradiation as reported by Lally et. al \cite{Lally}}
  \label{Lally Spectra}
\end{minipage}
\end{figure}

\begin{figure}[H]
\centering
\begin{minipage}{.49\textwidth}
  \centering
  \includegraphics[width=.95\textwidth]{Lit Review/Francini Fig 2.png}
  \caption{Emission spectra of TPB as a function of wavelength as represented by the three curves as reported by Francini et. al \cite{Francini}.}
  \label{Francini Spectra}
\end{minipage}\hfill
\begin{minipage}{.49\textwidth}
  \centering
  \includegraphics[width=0.95\textwidth]{Lit Review/Corning Fig 2 Top.png}
  \caption{Emission spectra of TBP from \SI{280}{nm} light irradiation as reported by Corning et. al \cite{jasmine_lidine}.  The temperature depended feature of the emission spectra is represented by the four curves.  Notice the second peak that emerges around \SI{400}{nm}}
  \label{Corning Spectra}
\end{minipage}
\end{figure}

External quantum efficiency has been found to be depended on both the thickness of the sample as well as the wavelength of the incident light as described by Lally et. al \cite{Lally}.  It is suggested that an optimal thickness of TPB to maximize the quantum efficiency and hence allow the most amount of light to be shifted to the visible spectrum is a thickness of \SI{0.07}{\mg\per\cm\squared}. It is also reported by Francini \cite{Francini} that as the thickness of the sample is increased, the emission spectrum of the TPB gradually is red-shifted.  It is suspected that this is due to the increased re-absorbance of photons alters the shape of the spectrum. 

\begin{figure}[H]
\centering
\begin{minipage}{.45\textwidth}
  \centering
  \includegraphics[width=1\linewidth]{Lit Review/Lally_5b.png}
  \caption{Quantum efficiency as a function of sample thickness using a \SI{175}{nm} source \cite{Lally}.}
  \label{Corning Quantum eff Thick}
\end{minipage}\hfill
\begin{minipage}{.45\textwidth}
  \centering
  \includegraphics[width=1\linewidth]{Lit Review/Lally_7b.png}
  \caption{Quantum efficiency of a \SI{0.07}{\mg\per\cm\squared} sample of TPB as a function of wavelength \cite{Lally}}
  \label{Corning Quantum Eff wave}
\end{minipage}
\end{figure}

When considering TPB as a candidate for use as a wavelength shifter, its optical properties such as index of refraction, optical conductivity, and absorption coefficient are useful to characterize the material. 
Information regarding absorption coefficients and refractive indices of TPB are reported by Graybill et. al \cite{Graybill}.  The method of application of TPB onto a glass thin film is that of spin coating which they claim to be of uniform thickness and have high optical transparency.  To preform this technique, TPB must be suspended in a polymer solution. Their findings indicate an absorption coefficient of less than \SI{0.001}{\per\cm} at a wavelength of \SI{435}{nm} but do not report an absorption coefficient in the ultraviolet spectrum.  They do however claim that the absorption coefficient and refractive index of TPB in the ultraviolet region must be equivalent of that of polymer solution \cite{Graybill}.  Thus the absorption coefficient and index of refraction of the polymer solution represent the maximum value for TPB and are displayed in the following figures \ref{Graybill absorption} and \ref{Graybill refraction}.

\begin{figure}[H]
\centering
\begin{minipage}{.45\textwidth}
  \centering
  \includegraphics[width=.9\linewidth]{Lit Review/Graybill_absorption.png}
  \caption{Absorption coefficients of a High Molecular Weight Polymer Solution as seen in the ultraviolet spectrum \cite{Graybill}.}
  \label{Graybill absorption}
\end{minipage}\hfill
\begin{minipage}{.45\textwidth}
  \centering
  \includegraphics[width=.9\linewidth]{Lit Review/Graybill_index_of_refraction.png}
  \caption{Index of refraction of a High Molecular Weight Polymer Solution as seen in the ultraviolet spectrum \cite{Graybill}}
  \label{Graybill refraction}
\end{minipage}
\end{figure}

While TPB has been reported to be an effective wavelength shifter, it has also been observed to scintillate \cite{Pollmann}.  The reported light yield of this scintillation is \SI{882}{photons\per\MeV} for alpha particle scintillation.  This reported light yield due to alpha particle scintillation is 5 times smaller than what is reported by G. Hull et. al. (see table 1 \cite{Hull} where \SI{5070}{photons\per\MeV} is reported.  In addition to this finding, it was reported by Standford et. al \cite{TPB2} that the scintillation lifetime of TPB depends on the type of radiation causing the scintillation.  This lifetime was reported to be on the order of \SI{1}{\ms}. A detailed process for describing the scintillation of TPB as a function of time is offered in appendix A of \cite{TPB2}.

The temperature dependence of the alpha induced scintillation was investigated by Veloce et. al. \cite{Veloce}. They report a method to discriminate these alpha induced scintillation from the nuclear and electronic recoils from LAr as seen in figure \ref{FPrompt} \cite{Veloce}.

 \begin{figure}[H]
    \centering
    \includegraphics[width=1\textwidth]{Lit Review/Veloce_FPromt.png}
  \caption{The plot of FPrompt vs Temperature allows for a clear discrimination between alpha induced backgrounds and electronic and nuclear recoils.}
    \label{FPrompt}
\end{figure}

The work of Segreto \cite{TPB1} unveiled that TPB not only emitted a "fast" light via the singlet state de-excitation but also a "slow" light via the triplet state de-excitation. The existence of a long-time constant is also reported by Veloce et. al. \cite{Veloce} are significant at temperatures above ~ \SI{50}{Kelvin}.
\subsubsection{Acrylic}

The re-emission  (luminescence) spectra were studied by J. M. Corning et. al \cite{LIDINE} and Tarasenko et. al \cite{Tarasenko}.  Their findings are reported in figure \ref{Corning_RPT} and \ref{Tarasneko_RPT}.  There is a clear discrepancy between the two spectra, noting the position of the peaks.  It is suggested that this could be caused by the the differing impurities in the samples and/or the method of excitation of the samples \cite{LIDINE}.

\begin{figure}{H}
    \centering{}
    \begin{minipage}{.45\textwidth}
        \centering{}
        \includegraphics[width=.9\linewidth]{Lit Review/Corning_RPT_emission.png}
        \caption{Re-emission spectra of RPT PMMA after irradiated by a \SI{280}{nm} light, measured at various temperatures.  A vertical offset of approximately 2.4 was applied to help distinguish between the trials.}
        \label{Corning_RPT}
    \end{minipage}\hfill
    \begin{minipage}{.45\textwidth}
        \centering
        \includegraphics[width=.9\linewidth]{Lit Review/Tarasenko_RPT_emission.png}
        \caption{Re-emission spectra of room temperature RPT PMMA when irradiated by a \SI{222}{nm} excilamp.}
        \label{Tarasneko_RPT}
    \end{minipage}
\end{figure}

Investigations into the optical characteristics of  various types of plastics were carried out by Piruska et. al \cite{Piruska} in 2005.  The different materials compared were PMMA, COC, PC, and PDMS.  These plastics were compared with glass made by BoroFloat for comparison as glass and plastic are both commonly used as a substrate for other material by dip or spin-coat application. The real part of the refractive indices of the materials of interest were studied and determined at various wavelengths and are found in table 1 of the article \cite{Piruska}.
To study and compare the autofluorescence of these materials, they were irradiated by a \SI{1}{milliwatt} laser for 60 seconds and varied the incident ray's wavelength.  The autofluorescence of all materials studied decreased as the incident ray's wavelength increased.  The BoroFloat glass was the least autofluorescent with PDMS being the most compariable to BoroFloat at \SI{633}{nm} \cite{Piruska} as seen in figure \ref{autoflourescence}.

 \begin{figure}[H]
    \centering
    \includegraphics[width=1\textwidth]{Lit Review/Piruska_autofluorescence.png}
  \caption{The autofluorescence of various plastic materials with BoroFloat seen in the top right corner.  As the incendent wavelength is increased, the autofluorescence decreases.}
    \label{autoflourescence}
\end{figure}

The autofluorescence property of these materials has been shown to decrease upon a sustained period of irradiation.  This effect was studied by Piruska et. al. by shining a \SI{488}{nm} \SI{1}{milliwatt} laser on PC for a period of 10 minutes and then repeating the experiment 12 hours later after leaving the plastic in a dark room \cite{Piruska}.  The autofluorescence decreased significantly as seen in figure \ref{bleaching} \cite{Piruska}.  This phenomenon, known as bleaching, is not perminate and has been shown to return to a state with stronger autofluorescence.  This is known as autofluorescence recovery \cite{Piruska}.

\begin{figure}[H]
    \centering
    \includegraphics[width=1\textwidth]{Lit Review/Piruska_bleach.png}
  \caption{The autoflourescence of PC as a function of irradiation time (left) and the autoflourescence of the same sample as a function of bleaching time after 12 hours without exposure to light soruces.}
    \label{bleaching}
\end{figure}
The photoluminescence response of RPT and Spartech acrylic (PMMA) was studied by G. R. Araujo \cite{RPT_LY} and was compared to the re-emission of TPB.  It was found that the re-emission intensity of TPB was much greater than the noise generate by the autoluminescence response of the acrylic as show in figure \ref{Araujo_emission}. It is reported that the cleaning procedure of the acrylic may play a critical role in the luminescence of these materials .  While it was reported that PMMA can function as a wavelength shifter, this effect is at most 0.2\% as effective as TPB between wavelengths of \SI{130}{nm} and \SI{250}{nm} and hence should have a minimal effect on the detectors \cite{RPT_LY}.

\begin{figure}{H}
    \centering
    \includegraphics[width=1\textwidth]{Lit Review/Araujo_emission_spectrum_TPB.png}
    \caption{Re-emission spectrum of TPB compared with the noise from RPT and PTFE acrylic.}
    \label{Araujo_emission}
    \end{figure}

The transmittance and attenuation of four samples of RPT were studied by Bodmer et. al. \cite{Bodmer}.  The transmittance of RPT, seen in figure \ref{Bodmer_transmittance}, tends to increase as wavelength increases, with a transmittance of approximately 69\% at \SI{440}{nm}, which is approximately the peak wavelength at which TPB re-emits light \cite{Bodmer}.

\begin{figure}[H]
    \centering
    \includegraphics[width=1\textwidth]{Lit Review/Bodmer_transmittance.png}
  \caption{The transmittance of four samples of RPT.  Notice the fourth sample has significantly lower transmission at smaller wavelengths. This sample is \SI{22.86}{cm} in diameter whereas the other three samples are \SI{10.0}{cm} in diameter.  While this fourth RPT sample is a UVA type, the other three are UVT type \cite{Bodmer}.}
    \label{Bodmer_transmittance}
\end{figure}
Attenuation length was also studied and is reported in figure \ref{Bodmer_attenuation} \cite{Bodmer}.  At the peak re-emission wavelegnth for TBP, the attenuation length of RPT is approximately \SI{2}{m}.

\begin{figure}[H]
    \centering
    \includegraphics[width=1\textwidth]{Lit Review/Bodmer_attenuation.png}
  \caption{Attenuation length vs wavelength (nm) for four samples of RPT.  As the wavelength increases, the attenuation tends to increase.}
    \label{Bodmer_attenuation}
\end{figure}

\subsection{Short time analysis results}

\subsection{Pauline's work}
\begin{itemize}
    \item Normalizing pulses to spe

Pulses are usually presented by plotting the amplitude versus time but another useful way to do it is to plot the number of photoelectrons per unit time versus time. This method enables to easily get an integral value without unit. In that case, if a fit is needed, it is also easy to calculate the $\chi^2$ value.
\\An example of this kind plot is presented Figure~\ref{normalizing_pulses_npe} for the TPB average pulse.
 \begin{figure}[h!]
    \centering
    \includegraphics[width=0.6\textwidth]{pauline/normalizing_pulses_npe.png}
  \caption{TPB average pulse : number of photoelectrons per unit time}
    \label{normalizing_pulses_npe}
\end{figure}

    \item Pulse shapes SPE, SPE/TPB, TPB
    
A pulse shape comparison have been carried out for the TPB, the TPB SPE and the SPE average pulses in order to study how the TPB fluorescence mechanism acts in time. 

The TPB SPE pulse corresponds to the signal after the absorption by the PMT photocathode of a single photon emitted by the TPB. The SPE pulse corresponds to the signal after the absorption by the PMT photocathode of a single photon emitted by a LED. 

Figure~\ref{TPB_TPBSPE} presents the average pulse of TPB and TPB SPE at two different scales. TPB data is displayed according to the left axis whereas the TPB SPE data amplitude scale is the one represented on the right axis. The time origin corresponds to the trigger time. TPB SPE average pulse has been also smoothed thanks to the application of an elliptic filter (through the \textit{scipy.signal} library). 
 \begin{figure}[h!]
    \centering
    \includegraphics[width=0.6\textwidth]{pauline/TPB_TPBSPE.png}
  \caption{TPB and TPB SPE average pulses}
    \label{TPB_TPBSPE}
\end{figure}
Without taking into account the high-frequency noise in the TPB SPE average pulse, the two shapes look very similar. A little bump is present around 0.905~$\mu s$ even if it looks more noticeable for the TPB SPE average pulse.

Figure~\ref{SPE_TPBSPE_1} presents the TPB SPE and SPE average pulses. The time origin corresponds to the trigger time for both.
A time shift can be noticed between the two peak starts. It is consistent that the TPB SPE light emission has a delay and that means that the TPB emission is not spontaneous. The shapes look similar but it will be easier to compare them with a time shift and a zoom as presented Figure~\ref{SPE_TPBSPE_2}.

\begin{figure}[h!]
\centering
\begin{minipage}{.45\textwidth}
  \centering
  \includegraphics[width=.9\linewidth]{pauline/SPE_TPBSPE_1.png}
  \caption{TPB SPE and SPE average pulses with trigger time at 0 $\mu$s}
  \label{SPE_TPBSPE_1}
\end{minipage}\hfill
\begin{minipage}{.45\textwidth}
  \centering
  \includegraphics[width=.9\linewidth]{pauline/SPE_TPBSPE_2.png}
  \caption{TPB SPE and SPE average pulses with a time shift}
  \label{SPE_TPBSPE_2}
\end{minipage}
\end{figure}

The average pulses look quite similar even if the TPB SPE peak is longer than the SPE ones. A small bump can be noticed at 105~ns but since it is present with and without the TPB, it means that it is not caused by the TPB, and is more likely a feature of the pulser, the PMT, or the electrical line.

    \item Fitting pulses

Those three average pulses have been fitted with a model described by the equation \ref{fitting_model}. This model contains two terms : the first one, a convolution of an exponential distribution with a normal distribution, represents the main peak while the second, a gaussian function, represents the little bump particularly noticed for the TPB SPE average (around 0.105 $\mu s$ Figure~\ref{TPB_TPBSPE}).

\begin{equation}
    f(x)=a_1 \textrm{conv\_expgauss}(x,\alpha_1, \mu_1, \sigma_1)+a_2 \textrm{gaussian}(x,\mu_2,\sigma_2)+C
    \label{fitting_model}
\end{equation}

$conv\_expgauss$ is the convolution of an exponential distribution and a normal distribution with $\alpha_1$ the exponential distribution parameter, and $\mu_1$ and $\sigma_1$ the mean and the standard deviation of the normal distribution. $gaussian$ is the normal probability density function where $\mu_2$ and $\sigma_2$ represent the mean and standard deviation of the normal distribution. $a_1$ and $a_2$ are related to the amplitude of each peak and $C$ is a constant.

The method for fits is the least squares one, which minimize the quantity S defined as :
\begin{equation}
    S=\sum_{i=1}^{n}\delta_i^2
\end{equation}
where $\delta_i=y_i-f(x_i)$ is the distance between the experimental value and the value predicted by the model and $n$ is the number of samples considered for the fit. 

Except $\mu_2$ and $\sigma_2$ which have fixed values (presented in Table~\ref{fixed_parameters}), all the parameters (a$_1$, $\alpha_1$,  $\mu_1$, $\sigma_1$, a$_2$, C) are free.

\begin{table}[h!]
\begin{center}
\begin{tabular}{l|cc}
              & $\mu_2$ (ns) & $\sigma_2$ (ns) \\ \hline
\textbf{SPE pulse   }  & 904          & 4.54            \\
\textbf{TPB SPE pulse} & 104          & 4.54            \\
\textbf{TPB pulse     }& 88           & 4.54           
\end{tabular}
\caption{Fixed parameters}
\label{fixed_parameters}
\end{center}
\end{table}

Figure~\ref{spe_fit}, \ref{tpbspe_fit} and \ref{tpb_fit} present the fit for the SPE pulse, the TPB SPE pulse and the TPB pulse respectively. In each figure, the results are presented in a first window with a linear vertical scale and in a second window with a logarithmic scale. The third window presents the evolution of $\delta^2$. The parameters fitted are presented Table~\ref{fitted_parameters}.

 \begin{figure}[h!]
    \centering
    \includegraphics[width=0.6\textwidth]{pauline/SPE_response_fit.png}
  \caption{Fit of SPE average pulse}
    \label{spe_fit}
\end{figure}

 \begin{figure}[h!]
    \centering
    \includegraphics[width=0.6\textwidth]{pauline/TPB_SPE_response_fit.png}
  \caption{Fit of TPB SPE average pulse}
    \label{tpbspe_fit}
\end{figure}

 \begin{figure}[h!]
    \centering
    \includegraphics[width=0.6\textwidth]{pauline/TPB_response_fit.png}
  \caption{Fit of TPB average pulse}
    \label{tpb_fit}
\end{figure}

\begin{table}[h!]
\begin{center}
\begin{tabular}{l|ccccccc}
  & a$_1$ (mV)            & $\alpha_1$ ($\mu$s$^{-1}$) & $\mu_1$ ($\mu$s)     & $\sigma_1$ ($\mu$s)  & a$_2$ (mV)            & C (mV)                & $S$ (V$^2$)        \\ \hline
\footnotesize{\textbf{SPE pulse}} & 0.150                & 296                      & 0.065                & 0.002                & 0.003                 & -0.036     &\textbf{5.65 x10$^{-5}$  }   \\
\footnotesize{\textbf{TPB SPE pulse}} & 0.154               & 250                      & 0.080                & 0.002                & 0.007                 & -0.072     & \textbf{1.39 x10$^{-3}$  } \\
\footnotesize{\textbf{TPB pulse}} & 12.6                & 252                      & 0.880                & 0.002                & 0.570                 & -2.04     & \textbf{1.68 x10$^{-2}$ }
\end{tabular}
\caption{Fitted parameters}
\label{fitted_parameters}
\end{center}
\end{table}

In those fitted parameters, one particularly important is $\alpha_1$ because it characterises the decay of each pulse since : $\alpha_1=\frac{1}{\tau}$ where $\tau$ is the decay time. Table~\ref{tau_fit} presents the values of the decay time for each pulse.

\begin{table}[h!]
\begin{center}
\begin{tabular}{l|c}
              & $\tau$ (ns) \\ \hline
\textbf{SPE pulse}     & 3.38        \\
\textbf{TPB SPE pulse} & 4.00        \\
\textbf{TPB pulse}     & 3.97       
\end{tabular}
\caption{Decay time $\tau$}
\label{tau_fit}
\end{center}
\end{table}
\end{itemize}

These values confirm that the TPB fluorescence show a slower decay than the response of a photon emitted directly by a LED.

\subsection{Hicham's late light}

In our study, TPB and RPT runs both showed lower-amplitude and delayed light after prompt light main peak. This observed late light has a decreasing amplitude with time and could have been due to TPB and RPT samples late luminescence.
\\
\\
We analysed this late light and found a way to get the number of photoelectrons detected by getting rid of the electronic noise and taking into account vertical ranges. Then, we were able to study the behaviour of this late light with different sample temperatures. Whatever the temperature of the sample is, we found a relatively stable number of photoelectrons in late light. Small variations were found to be due to environmental conditions.
\\
\\
On Fig.~\ref{fig:63p4}, we compare late light detected by the PMT with a TPB sample, a RPT sample and without sample. Run with no sample is only 10 microseconds long so the three runs are showed in order to have main prompt peaks at the same time. Then, we should only compare curves between 17 and 27 microseconds. The average amplitudes are showed in Volts and per event to get rid of the number of events and the vertical range of each run.

\begin{figure}[H]
\begin{center}
\includegraphics[width=11cm]{63p4.png}
\caption{\label{fig:63p4}Average amplitude per event with RPT sample, TPB sample and without sample - 300K}

\end{center}
\end{figure}

On Fig.~\ref{fig:63p4}, we can see that TPB sample and RPT sample curves, respectively orange and blue curves have similar shapes for later light, the difference for earlier late light is due to afterpulsing effect in TPB run.

If we compare TPB run and no sample run (green curve), we can see that both late lights are very close to each other and the shapes are almost exactly the same. The small difference could be due to the noise we see in pretrigger area in the run without sample.

We can conclude from this study that the observed late light observed in TPB and RPT runs is not due to the sample. It is instrumental light, most likely due to visible light from LED being directly detected by the photo-multiplier tube.

If TPB and RPT are responsible for any late light, it is negligible compared to instrumental light and afterpulsing. Late light would have a lower amplitude than sensitivity of the experiment.

\subsection{Light Yield Measurements by Jasmine}

For purpose of comparison.

\begin{figure}[htp]
    \centering
    \resizebox{\textwidth}{!}{
    \begin{tabular}{cc}
        \includegraphics{TPB2_lightyield_mu.pdf} & \includegraphics{TPB2_lightyield_pes.pdf} \\
    \end{tabular}}
    \caption{Light yield of the TPB sample in terms of average integral (left) and estimated number of PEs (right).}
\end{figure}

\begin{figure}[htp]
    \centering
    \resizebox{\textwidth}{!}{
    \begin{tabular}{cc}
        \includegraphics{RPT2_lightyield_mu.pdf} & \includegraphics{RPT2_lightyield_pes.pdf} \\
    \end{tabular}}
    \caption{Light yield of the RPT sample in terms of average integral (left) and estimated number of PEs (right).}
\end{figure}

\begin{figure}[htp]
    \centering
    \includegraphics[width=0.8\textwidth]{TPB2vsRPT2_lightyield.pdf}
    \caption{Relative light yield of TPB to RPT, using estimated PE values.}
\end{figure}

\begin{figure}[htp]
    \centering
    \includegraphics[width=0.8\textwidth]{TPB2vsRPT2_lightyield_2.pdf}
    \caption{Relative light yield of TPB to RPT, using average integral values.}
\end{figure}

\newpage
\subsection{Setup and Fit Parameters Stability by Vitaliy}

\begin{figure}[H]
    \centering
    \includegraphics[scale=0.3]{RPT/RPT_LY(50ns).pdf}
    \caption{RPT detected light yield vs temperature}
    \label{fig:RPT_LY_}
\end{figure}

\begin{figure}[H]
    \centering
    \includegraphics[scale=0.3]{Setup and Fit Parameters Stability/RPTspe.pdf}
    \caption{Spe on temperature.}
\end{figure}

\begin{figure}[H]
    \centering
    \includegraphics[scale=0.3]{Setup and Fit Parameters Stability/Spe_noise_corr.pdf}
    \caption{Spe on x0.}
\end{figure}

\begin{figure}[H]
    \centering
    \includegraphics[scale=0.3]{Setup and Fit Parameters Stability/x0_s0_corr.pdf}
    \caption{s0 on x0.}
\end{figure}

\begin{figure}[H]
    \centering
    \includegraphics[scale=0.3]{Setup and Fit Parameters Stability/Average_300_250.pdf}
    \caption{Average traces 300K 250K.}
\end{figure}

\begin{figure}[H]
    \centering
    \includegraphics[scale=0.3]{Setup and Fit Parameters Stability/Average_100_77.pdf}
    \caption{Average traces 100K 77K.}
\end{figure}

\begin{figure}[H]
    \centering
    \includegraphics[scale=0.3]{Setup and Fit Parameters Stability/noise_distr.pdf}
    \caption{Distributions of absolute values integrals in 850-865ns}
\end{figure}

\begin{figure}[H]
    \centering
    \includegraphics[scale=0.3]{Setup and Fit Parameters Stability/noise_plot.pdf}
    \caption{Average absolute values integrals of noise vs Temperature}
\end{figure}

\begin{figure}[H]
    \centering
    \includegraphics[scale=0.3]{Setup and Fit Parameters Stability/noise_std.pdf}
    \caption{Correlation between standard deviations of baseline and average absolute values integrals}
\end{figure}

\begin{figure}[H]
    \centering
    \includegraphics[scale=0.3]{Setup and Fit Parameters Stability/RPT_LY(50nm)_noise.pdf}
    \caption{RPT detected light yield with new errorbars}
\end{figure}

\subsection{Matthieu's Radioluminescent Pulse}

A block of PMMA acrylic was exposed to a St90/Y90 beta emitting source.  The acrylic was then observed re-emit photons with a peak wavelength of approximately $\sim 425 nm$ exhibited in figure~\ref{radiolum}.  While the spectum does show a definite peak, the resolution is quite small, and hence there is minimal response from the sample.

Strontium-90 emits an electron with $\sim 0.546 MeV$ and decays into Yittrium-90 which beta decays into stable zirconium-90, with energy $\sim 2.28 MeV$.  These electrons could travel through the acrylic faster than the speed of light in the medium, producing Cherenkov radiation, which in turn could be absorbed and re-emitted as visible light (source?).  This process is different from the mechanisms behind radioluminescence (source and more detail needed). Radioluminescence is observing the wavelength spectra from scintillation.

\begin{figure}[H]
    \centering
    \includegraphics[scale=0.8]{Radiolum_PMMA.png}
    \caption{Radioluminescent spectra of PMMA acrylic with its transmission}
    \label{radiolum}
\end{figure}

\subsection{Comparing spectra to literature}
\begin{figure}[H]
        \centering
        \includegraphics[width=0.6\textwidth]{spectra/rpt_literature_spectra.pdf}
        \caption{RPT spectrum from this work compared to data presented in \cite{Tarasenko}}
        \label{fig:rpt_lit_spec}
\end{figure}

\begin{figure}[H]
        \centering
        \includegraphics[width=0.98\textwidth]{spectra/tpb_literature_spectra.pdf}
        \caption{Comparing the TPB spectra at 300 K and 87 K from this work and from  \cite{Francini}}
        \label{fig:tpb_lit_spec}
\end{figure}

\newpage

%\endif
